# Supplementary material for: Quantum Christoffel Nonlinear Magnetization
Source: arXiv:2602.03597 source file (2026-02-03)
Supplement: Supplementary file 1 [file Supp.pdf]

# Supplemental Material for
# "Quantum Christoffel Nonlinear Magnetization"

Xiao-Bin Qiang,[1,*] Xiaoxiong Liu,[1,*] Hai-Zhou Lu,[1,2,†] and X. C. Xie[3,4,5]

[1] *State Key Laboratory of Quantum Functional Materials, Department of Physics, and Guangdong Basic Research Center of Excellence for Quantum Science, Southern University of Science and Technology (SUSTech), Shenzhen 518055, China*
[2] *Quantum Science Center of Guangdong-Hong Kong-Macao Greater Bay Area (Guangdong), Shenzhen 518045, China*
[3] *International Center for Quantum Materials, School of Physics, Peking University, Beijing100871, China*
[4] *Interdisciplinary Center for Theoretical Physics and Information Sciences (ICTPIS), Fudan University, Shanghai 200433, China*
[5] *Hefei National Laboratory, Hefei 230088, China*

(Dated: February 3, 2026)

This Supplemental Material provides detailed derivations and supporting calculations, which includes Refs. [1–9].

**CONTENTS**

SI. Calculation of orbital magnetic moment correction — S1
A. Wave packet and field induced Berry connection — S1
B. Electric field induced correction of orbital magnetic moment — S5
C. Gauge invariant formalisms — S5

SII. Calculation of distribution function — S7

SIII. Calculation of nonlinear magnetization coefficient — S7

SIV. Particle-hole symmetry and solo of quantum Christoffel symbol — S9
A. Two-band system — S9
B. 2D massive Dirac model — S11

SV. Symmetry analysis and 2D material candidates — S11

SVI. Comparison with spin contribution — S12
A. Nonlinear spin magnetization — S12
B. First principle calculations for $BiF_3$ — S14

References — S14

## SI. CALCULATION OF ORBITAL MAGNETIC MOMENT CORRECTION

### A. Wave packet and field induced Berry connection

By considering the magnetic field as perturbation, the local Hamiltonian is

$$\mathcal{H}_c = \mathcal{H}_0\left[\mathbf{p} + e\mathbf{A}\left(\mathbf{r}_c, t\right), \mathbf{r}\right], \tag{S1}$$

where $\mathbf{r}_c$ is the center of mass of the wave packet, $\mathbf{A}$ is the magnetic vector potential, and the magnetic field is decided by $\mathbf{B} = \nabla \times \mathbf{A}$. The unperturbed Hamiltonian $\mathcal{H}_0$ satisfies the eigenequation

$$\mathcal{H}_0(\mathbf{p}, \mathbf{r}) \left|\psi_\nu(\mathbf{k})\right\rangle = \varepsilon_\nu(\mathbf{k}) \left|\psi_\nu(\mathbf{k})\right\rangle, \tag{S2}$$

* These authors contributed equally to this work.
† Corresponding author: luhz@sustech.edu.cn

where $\nu$ and $\mathbf{k}$ are band-index and crystal momentum ($\hbar\mathbf{k}$ is the eigenvalue of momentum operator $\mathbf{p}$). By replacing $\mathbf{k}$ with the gauge invariant crystal momentum $\mathbf{k}+(e/\hbar)\mathbf{A}$, the form of eigenenergy remains unchanged $\varepsilon_\nu^{(0)}=\varepsilon_\nu(\mathbf{k})$, the eigenstate remains the Bloch function

$$|\psi_\nu(\mathbf{k})\rangle = e^{i\mathbf{k}\cdot\mathbf{r}}|\nu(\mathbf{k})\rangle. \tag{S3}$$

The first-order correction to the local Hamiltonian $\mathcal{H}_c$ is

$$\mathcal{H}_1=\frac{e}{2}\mathbf{B}\cdot\left[(\mathbf{r}-\mathbf{r}_c)\times\mathbf{v}\right]. \tag{S4}$$

Up to the first-order in field, the Hamiltonian is $\mathcal{H}=\mathcal{H}_c+\mathcal{H}_1$, the energy is $\tilde{\varepsilon}_\nu=\varepsilon_\nu^{(0)}+\varepsilon_\nu^{(1)}$ with $\varepsilon_\nu^{(1)}=-\mathbf{B}\cdot\mathbf{m}_\nu$, where $\mathbf{m}_\nu$ is the intra-band orbital magnetic moment. We construct the wave packet as follows

$$|\tilde{W}\rangle = e^{-i(e/\hbar)\mathbf{A}\cdot\mathbf{r}}\int d\mathbf{k}\Big[w_\nu(\mathbf{k})|\psi_\nu(\mathbf{k})\rangle+\sum_{\mu\neq\nu}w_\mu^{(1)}(\mathbf{k})|\psi_\mu(\mathbf{k})\rangle\Big], \tag{S5}$$

where $w_\nu$ is the zeroth-order amplitude with $|w_\nu|^2\simeq\delta(\mathbf{k}-\mathbf{k}_c)$, $w_\nu^{(1)}$ incorporates the inter-band mixing and is the first-order in external field. An additional phase factor has been added to locally gauge away the vector potential at the center of the wave packet. Coefficients $w_\nu$ and $w_\nu^{(1)}$ are not independent, their relation can identified by the time-dependent Schrödinger equation $i\hbar\partial_t|\tilde{W}\rangle=\mathcal{H}|\tilde{W}\rangle$. Firstly, the dynamical part is

$$\begin{aligned}
i\hbar\partial_t|\tilde{W}\rangle &= e(\partial_{\mathbf{r}_c}\mathbf{A}\dot{\mathbf{r}}_c)\cdot\mathbf{r}|\tilde{W}\rangle + e^{-i(e/\hbar)\mathbf{A}\cdot\mathbf{r}}i\hbar\partial_t\int d\mathbf{k}'\Big[w_\nu|\psi_\nu\rangle+\sum_{\mu\neq\nu}w_\mu^{(1)}|\psi_\mu\rangle\Big]\\
&=\frac{e}{2}(\mathbf{B}\times\dot{\mathbf{r}}_c)\cdot\mathbf{r}|\tilde{W}\rangle + e^{-i(e/\hbar)\mathbf{A}\cdot\mathbf{r}}\tilde{\varepsilon}_\nu\int d\mathbf{k}'\Big[w_\nu|\psi_\nu\rangle+\sum_{\mu\neq\nu}w_\mu^{(1)}|\psi_\mu\rangle\Big],
\end{aligned} \tag{S6}$$

where we have used the relation $\dot{\mathbf{r}}_c\cdot(\partial_{\mathbf{r}_c}\mathbf{A})=\mathbf{B}\times\dot{\mathbf{r}}_c/2$. To obtain the first-order amplitude $w_\mu^{(1)}$, we take the inner product with $\langle\psi_\rho(\mathbf{k})|e^{i(e/\hbar)\mathbf{A}\cdot\mathbf{r}}$ with $\rho\neq\nu$,

$$\begin{aligned}
\langle\psi_\rho(\mathbf{k})|e^{i(e/\hbar)\mathbf{A}\cdot\mathbf{r}}i\hbar\partial_t|\tilde{W}\rangle =&\frac{e}{2}(\mathbf{B}\times\dot{\mathbf{r}}_c)\cdot\int d\mathbf{k}'\Big[\langle\psi_\rho(\mathbf{k})|\mathbf{r}|\psi_\nu(\mathbf{k}')\rangle w_\nu+\sum_{m\neq n}\langle\psi_\rho(\mathbf{k})\mid\mathbf{r}|\psi_\mu(\mathbf{k}')\rangle w_\mu^{(1)}\Big]\\
&+\int d\mathbf{k}'\Big[\tilde{\varepsilon}_\nu\langle\psi_\rho(\mathbf{k})\mid\psi_\nu(\mathbf{k}')\rangle w_\nu+\sum_{\mu\neq\nu}\tilde{\varepsilon}_\nu\langle\psi_\rho(\mathbf{k})\mid\psi_\mu(\mathbf{k}')\rangle w_\mu^{(1)}\Big]\\
=&\frac{e}{2}(\mathbf{B}\times\dot{\mathbf{r}}_c)\cdot\int d\mathbf{k}'\Big[(i\delta_{\rho\nu}\partial_{\mathbf{k}}+\boldsymbol{\mathcal{A}}_{\rho\nu})\delta(\mathbf{k}'-\mathbf{k})w_\nu+\sum_{\mu\neq\nu}\langle\psi_\rho(\mathbf{k})\mid\mathbf{r}|\psi_\mu(\mathbf{k}')\rangle w_\mu^{(1)}\Big]\\
&+\int d\mathbf{k}'\Big[\tilde{\varepsilon}_\nu w_\nu\delta_{\rho\nu}+\sum_{\mu\neq\nu}\tilde{\varepsilon}_\nu w_\mu^{(1)}\delta_{\rho\mu}\Big]\delta(\mathbf{k}'-\mathbf{k})\\
\simeq&\frac{e}{2}(\mathbf{B}\times\dot{\mathbf{r}}_c)\cdot\boldsymbol{\mathcal{A}}_{\rho\nu}w_\nu+\varepsilon_\nu w_\rho^{(1)},
\end{aligned} \tag{S7}$$

where $\boldsymbol{\mathcal{A}}_{\mu\nu}=\langle\mu|i\partial_{\mathbf{k}}|\nu\rangle$ is the inter-band Berry connection, the terms with $\mathbf{B}w_\nu^{(1)}$ have been dropped since $w_\nu^{(1)}$ is already of first order in field [in addition the field correction energy $\tilde{\varepsilon}_\nu w_\nu^{(1)}=(\varepsilon_\nu-\mathbf{B}\cdot\mathbf{m}_\nu)w_\nu^{(1)}\simeq\varepsilon_\nu w_\nu^{(1)}$], and the identity

$$\langle\psi_\mu(\mathbf{k})|\mathbf{r}|\psi_\nu(\mathbf{k}')\rangle=(i\delta_{\mu\nu}\partial_{\mathbf{k}}+\boldsymbol{\mathcal{A}}_{\mu\nu})\,\delta(\mathbf{k}'-\mathbf{k}) \tag{S8}$$

has been used.

The energetic part of Schrödinger equation is

$$\begin{aligned}
\mathcal{H}|\tilde{W}\rangle &= e^{-i(e/\hbar)\mathbf{A}\cdot\mathbf{r}}\int d\mathbf{k}'\Big[\mathcal{H}_c w_\nu|\psi_\nu\rangle+\sum_{m\neq n}\mathcal{H}_c w_\mu^{(1)}|\psi_\mu\rangle+\mathcal{H}_1 w_\nu|\psi_\nu\rangle+\sum_{\mu\neq\nu}\mathcal{H}_1 w_\mu^{(1)}|\psi_\mu\Big]\\
&= e^{-i(e/\hbar)\mathbf{A}\cdot\mathbf{r}}\int d\mathbf{k}'\Big[\varepsilon_\nu w_\nu|\psi_\nu\rangle+\sum_{\mu\neq\nu}\varepsilon_\mu w_\mu^{(1)}|\psi_\mu\rangle+\mathcal{H}_1 w_\nu|\psi_\nu\rangle+\sum_{m\neq n}\mathcal{H}_1 w_\mu^{(1)}|\psi_\mu\rangle\Big]\\
&= e^{-i(e/\hbar)\mathbf{A}\cdot\mathbf{r}}\int d\mathbf{k}'\Big[(\varepsilon_\nu+\mathcal{H}_1)w_\nu|\psi_\nu\rangle+\sum_{\mu\neq\nu}(\varepsilon_\mu+\mathcal{H}_1)w_\mu^{(1)}|\psi_\mu\rangle\Big].
\end{aligned} \tag{S9}$$

Similarly, by taking the inner product with $\langle\psi_\rho(\mathbf{k})|e^{i(e/\hbar)\mathbf{A}\cdot\mathbf{r}}$ with $\rho\neq\nu$, we have

$$\begin{aligned}\langle\psi_\rho(\mathbf{k})|e^{i(e/\hbar)\mathbf{A}\cdot\mathbf{r}}\mathcal{H}|\tilde{W}\rangle =&\varepsilon_\nu w_\nu\delta_{\rho\nu}+\int d\mathbf{k}'\left[\langle\psi_\rho(\mathbf{k})|\mathcal{H}_1|\psi_\nu(\mathbf{k}')\rangle\right]w_\nu+\sum_{\mu\neq\nu}\Big[\varepsilon_\mu\delta_{\rho\mu}+\int d\mathbf{k}'\langle\psi_\rho(\mathbf{k})|\mathcal{H}_1|\psi_\mu(\mathbf{k}')\rangle\Big]w_\mu^{(1)}\\ =&\int d\mathbf{k}'\Big[\frac{e}{2}\mathbf{B}\cdot\langle\psi_\rho(\mathbf{k})|(\mathbf{r}-\mathbf{r}_c)\times\mathbf{v}|\psi_\nu(\mathbf{k}')\rangle\Big]w_\nu+\varepsilon_\rho w_\rho^{(1)}+\sum_{\mu\neq\nu}\int d\mathbf{k}'\langle\psi_\rho(\mathbf{k})|\mathcal{H}_1|\psi_\mu(\mathbf{k}')\rangle w_\mu^{(1)}\\ \simeq&\varepsilon_\rho w_\rho^{(1)}+\frac{e}{2}\mathbf{B}\times(i\partial_\mathbf{k}+\boldsymbol{\mathcal{A}}_\nu-\mathbf{r}_c)w_\nu\cdot\mathbf{v}_{\rho\nu}-\frac{e}{2}\mathbf{B}\cdot\sum_{\mu\neq\nu}\mathbf{v}_{\rho\mu}\times\boldsymbol{\mathcal{A}}_{\mu\nu}w_\nu,\end{aligned}\tag{S10}$$

where $\mathbf{v}_{\mu\nu}=\langle\mu|\mathbf{v}|\nu\rangle$ is the matrix element of velocity, and we have again dropped the term with $\mathcal{H}_1w_\nu^{(1)}$ ($\sim\mathbf{B}w_\nu^{(1)}$). We remark that

$$\begin{aligned}&\int d\mathbf{k}'\langle\psi_\rho(\mathbf{k})|(\mathbf{r}-\mathbf{r}_c)\times\mathbf{v}|\psi_\nu(\mathbf{k}')\rangle w_\nu\\ =&\int d\mathbf{k}'\langle\psi_\rho(\mathbf{k})|\mathbf{r}\times\mathbf{v}|\psi_\nu(\mathbf{k}')\rangle w_\nu-\int d\mathbf{r}\int d\mathbf{k}'e^{i(\mathbf{k}'-\mathbf{k})\cdot\mathbf{r}}\mathbf{r}_c\times\langle l(\mathbf{k})|\mathbf{v}|\nu(\mathbf{k}')\rangle w_\nu\\ =&\sum_\mu\int d\mathbf{k}'\langle\psi_\rho(\mathbf{k})|\mathbf{r}|\psi_\mu(\mathbf{k}')\rangle\times\langle\psi_\mu(\mathbf{k}')|\mathbf{v}|\psi_\nu(\mathbf{k}')\rangle w_\nu-\mathbf{r}_c\times\mathbf{v}_{\rho\nu}w_\nu\\ =&\sum_\mu\int d\mathbf{k}'(i\delta_{\rho\mu}\partial_\mathbf{k}+\boldsymbol{\mathcal{A}}_{\rho\mu})\delta(\mathbf{k}'-\mathbf{k})\times\mathbf{v}_{mn}w_\nu-\mathbf{r}_c\times\mathbf{v}_{\rho\nu}w_\nu\\ =&(i\partial_\mathbf{k}-\mathbf{r}_c)w_\nu\times\mathbf{v}_{\rho\nu}+\sum_\mu\boldsymbol{\mathcal{A}}_{\rho\mu}\times\mathbf{v}_{\mu\nu}w_\nu\\ =&(i\partial_\mathbf{k}+\boldsymbol{\mathcal{A}}_\nu-\mathbf{r}_c)w_\nu\times\mathbf{v}_{\rho\nu}-\sum_{\mu\neq\nu}\mathbf{v}_{\rho\mu}\times\boldsymbol{\mathcal{A}}_{\mu\nu}w_\nu,\end{aligned}\tag{S11}$$

where we have used the relation

$$\begin{aligned}\sum_\mu\boldsymbol{\mathcal{A}}_{\rho\mu}\times\mathbf{v}_{\mu\nu}=&\sum_\mu\langle\rho|i\partial_\mathbf{k}|\mu\rangle\times\langle\mu|\mathbf{v}|\nu\rangle\\ =&-\sum_\mu\langle\rho|\mathbf{v}|\mu\rangle\times\langle\mu|i\partial_\mathbf{k}|\nu\rangle\\ =&-\sum_{\mu\neq\nu}\mathbf{v}_{\rho\mu}\times\boldsymbol{\mathcal{A}}_{\mu\nu}+\boldsymbol{\mathcal{A}}_\nu\times\mathbf{v}_{\rho\nu}.\end{aligned}\tag{S12}$$

Accordingly, the Schrödinger equation gives

$$\begin{aligned}&\frac{e}{2}(\mathbf{B}\times\dot{\mathbf{r}}_c)\cdot\boldsymbol{\mathcal{A}}_{\rho\nu}w_\nu+\varepsilon_\nu w_\rho^{(1)}=\varepsilon_\rho w_\rho^{(1)}+\frac{e}{2}\mathbf{B}\times(i\partial_\mathbf{k}+\boldsymbol{\mathcal{A}}_\nu-\mathbf{r}_c)w_\nu\cdot\mathbf{v}_{\rho\nu}-\frac{e}{2}\mathbf{B}\cdot\sum_{\mu\neq\nu}\mathbf{v}_{\rho\mu}\times\boldsymbol{\mathcal{A}}_{\mu\nu}w_\nu,\\ \Rightarrow\quad&(\varepsilon_\nu-\varepsilon_\rho)w_\rho^{(1)}=-\frac{e}{2}\mathbf{B}\cdot\sum_{\mu\neq\nu}\mathbf{v}_{\rho\mu}\times\boldsymbol{\mathcal{A}}_{\mu\nu}w_\nu-\frac{e}{2}(\mathbf{B}\times\dot{\mathbf{r}}_c)\cdot\boldsymbol{\mathcal{A}}_{\rho\nu}w_\nu+\frac{e}{2}\mathbf{B}\times(i\partial_\mathbf{k}+\boldsymbol{\mathcal{A}}_\nu-\mathbf{r}_c)w_\nu\cdot\mathbf{v}_{\rho\nu},\\ \Rightarrow\quad&(\varepsilon_\nu-\varepsilon_\rho)w_\rho^{(1)}=-\frac{e}{2}\mathbf{B}\cdot\sum_{\mu\neq\nu}(\mathbf{v}_{\rho\mu}+\mathbf{v}_\nu\delta_{\rho\mu})\times\boldsymbol{\mathcal{A}}_{\mu\nu}w_\nu+\frac{e}{2}\mathbf{B}\times(i\partial_\mathbf{k}+\boldsymbol{\mathcal{A}}_\nu-\mathbf{r}_c)w_\nu\cdot\mathbf{v}_{\rho\nu},\\ \Rightarrow\quad&w_\rho^{(1)}=\frac{1}{\varepsilon_\nu-\varepsilon_\rho}\Big[-\frac{e}{2}\mathbf{B}\cdot\sum_{\mu\neq\nu}(\mathbf{v}_{\rho\mu}+\mathbf{v}_\nu\delta_{\rho\mu})\times\boldsymbol{\mathcal{A}}_{\mu\nu}w_\nu+\frac{e}{2}\mathbf{B}\times(i\partial_\mathbf{k}+\boldsymbol{\mathcal{A}}_\nu-\mathbf{r}_c)w_\nu\cdot\mathbf{v}_{\rho\nu}\Big].\end{aligned}\tag{S13}$$

By defining a dimensionless quantity

$$\mathcal{C}_{\mu\nu}=\frac{-\mathbf{B}\cdot\mathbf{m}_{\mu\nu}}{\varepsilon_\nu-\varepsilon_\mu}\tag{S14}$$

with inter-band element of the orbital magnetic moment

$$\mathbf{m}_{\mu\nu}=\frac{e}{2}\sum_{\rho\neq\nu}(\mathbf{v}_{\mu\rho}+\mathbf{v}_\nu\delta_{\rho\mu})\times\boldsymbol{\mathcal{A}}_{\rho\nu},\tag{S15}$$

and using the relation [for the last term of Eq. (S13)]

$$\begin{aligned}\mathbf{v}_{\mu\nu} &= \langle \mu\,|\partial_{\mathbf{k}}\mathcal{H}/\hbar|\,\nu\rangle \\ &= -\frac{i}{\hbar}\langle \mu\,|i\partial_{\mathbf{k}}|\,\nu\rangle\,(\varepsilon_\nu-\varepsilon_\mu) \\ &= -\frac{i}{\hbar}\boldsymbol{\mathcal{A}}_{\mu\nu}\,(\varepsilon_\nu-\varepsilon_\mu)\,,\end{aligned} \tag{S16}$$

the coefficient $w_\mu^{(1)}$ is formally given by

$$w_\mu^{(1)} = \mathcal{C}_{\mu\nu}w_\nu - \frac{ie}{2\hbar}\left[\mathbf{B}\times(i\partial_{\mathbf{k}}+\boldsymbol{\mathcal{A}}_\nu-\mathbf{r}_c)\,w_\nu\right]\cdot\boldsymbol{\mathcal{A}}_{\mu\nu}. \tag{S17}$$

By substituting $w_\nu^{(1)}$ into Eq. (S5), we completely construct the wave packet

$$\begin{aligned}|\tilde{W}\rangle &= e^{-i(e/\hbar)\mathbf{A}\cdot\mathbf{r}}\int d\mathbf{k}\Big[w_\nu(\mathbf{k})|\psi_\nu\rangle + \sum_{\mu\neq\nu} w_\mu^{(1)}|\psi_\mu\rangle\Big] \\ &= e^{-i(e/\hbar)\mathbf{A}\cdot\mathbf{r}}\int d\mathbf{k}\Big\{w_\nu|\psi_\nu\rangle + \sum_{\mu\neq\nu}\mathcal{C}_{\mu\nu}w_\nu - \frac{i}{2}\frac{e}{\hbar}\big[\mathbf{B}\times(i\partial_{\mathbf{k}}+\boldsymbol{\mathcal{A}}_\nu-\mathbf{r}_c)w_\nu\big]\cdot\sum_{m\neq n}\boldsymbol{\mathcal{A}}_{\mu\nu}|\psi_\mu\rangle\Big\}.\end{aligned} \tag{S18}$$

With this field corrected wave packet, the center of mass changes as

$$\begin{aligned}\langle\tilde{W}|\mathbf{r}|\tilde{W}\rangle &= \langle W|\mathbf{r}|W\rangle + \sum_{\mu\neq\nu}\int d\mathbf{k}\int d\mathbf{k}'w_\nu^*(\mathbf{k})w_\mu^{(1)}(\mathbf{k}')\langle\psi_\nu(\mathbf{k})|\mathbf{r}|\psi_\mu(\mathbf{k}')\rangle + \text{c.c.} \\ &= \mathbf{r}_c + \sum_{\mu\neq\nu}\int d\mathbf{k}\int d\mathbf{k}'w_\nu^*(\mathbf{k})w_\mu^{(1)}(\mathbf{k}')\left(i\delta_{\nu\mu}\partial_{\mathbf{k}}+\boldsymbol{\mathcal{A}}_{\nu\mu}\right)\delta\left(\mathbf{k}'-\mathbf{k}\right) + \text{c.c.} \\ &= \mathbf{r}_c + \sum_{\mu\neq\nu}\int d\mathbf{k}w_\nu^* w_\mu^{(1)}\boldsymbol{\mathcal{A}}_{\nu\mu} + \text{c.c.}.\end{aligned} \tag{S19}$$

The unperturbed center of mass has been given by $\mathbf{r}_c$=$\partial_{\mathbf{k}}\gamma_\nu+\boldsymbol{\mathcal{A}}_\nu$. The second term represents the additional shift to the center of mass due to the external magnetic field $\mathbf{B}$, which we refer to as the field induced Berry connection and label it by $\boldsymbol{\mathcal{A}}_\nu^{(1)}$. By using the expression of $w_\nu^{(1)}$ [Eq. (S17)], $\boldsymbol{\mathcal{A}}_\nu^{(1)}$ can be further calculated as follows

$$\begin{aligned}\boldsymbol{\mathcal{A}}_\nu^{(1)} &= \sum_{\mu\neq\nu}\int d\mathbf{k}w_\nu^* w_\mu^{(1)}\boldsymbol{\mathcal{A}}_{\nu\mu}+\text{c.c.} \\ &= \sum_{\mu\neq\nu}\int d\mathbf{k}w_\nu^*\Big\{\mathcal{C}_{\mu\nu}w_\nu - \frac{ie}{2\hbar}\big[\mathbf{B}\times(i\partial_{\mathbf{k}}+\boldsymbol{\mathcal{A}}_\nu-\mathbf{r}_c)w_\nu\big]\cdot\boldsymbol{\mathcal{A}}_{\mu\nu}\Big\}\boldsymbol{\mathcal{A}}_{\nu\mu}+\text{c.c.} \\ &= \sum_{\mu\neq\nu}\int d\mathbf{k}|w_\nu|^2\boldsymbol{\mathcal{A}}_{\nu\mu}\mathcal{C}_{\mu\nu} - \frac{ie}{2\hbar}\sum_{\mu\neq\nu}\int d\mathbf{k}w_\nu^*\big[\mathbf{B}\times(i\partial_{\mathbf{k}}+\boldsymbol{\mathcal{A}}_\nu-\mathbf{r}_c)w_\nu\big]_i\mathcal{A}^i_{\mu\nu}\boldsymbol{\mathcal{A}}_{\nu\mu}+\text{c.c.} \\ &= \sum_{\mu\neq\nu}\boldsymbol{\mathcal{A}}_{\nu\mu}\mathcal{C}_{\mu\nu} + \frac{e}{2\hbar}\sum_{\mu\neq\nu}\int d\mathbf{k}w_\nu^*\big(\mathbf{B}\times\partial_{\mathbf{k}}|w_\nu|\big)_i e^{-i\gamma_\nu}\mathcal{A}^i_{\mu\nu}\boldsymbol{\mathcal{A}}_{\nu\mu} \\ &\quad - \frac{ie}{2\hbar}\sum_{\mu\neq\nu}\int d\mathbf{k}w_\nu^* w_\nu\big[\mathbf{B}\times(\partial_{\mathbf{k}}\gamma_\nu+\boldsymbol{\mathcal{A}}_\nu-\mathbf{r}_c)\big]_i\mathcal{A}^i_{\mu\nu}\boldsymbol{\mathcal{A}}_{\nu\mu}+\text{c.c.} \\ &= \sum_{\mu\neq\nu}\boldsymbol{\mathcal{A}}_{\nu\mu}\mathcal{C}_{\mu\nu} + \frac{e}{4\hbar}\sum_{\mu\neq\nu}\int d\mathbf{k}\big(\mathbf{B}\times\partial_{\mathbf{k}}|w_\nu|^2\big)_i\mathcal{A}^i_{\mu\nu}\boldsymbol{\mathcal{A}}_{\nu\mu}+\text{c.c.} \\ &= 2\text{Re}\sum_{\mu\neq\nu}\boldsymbol{\mathcal{A}}_{\nu\mu}\mathcal{C}_{\mu\nu} - \frac{e}{2\hbar}\text{Re}\sum_{\mu\neq\nu}\big(\mathbf{B}\times\partial_{\mathbf{k}}\big)_i\mathcal{A}^i_{\mu\nu}\boldsymbol{\mathcal{A}}_{\nu\mu}.\end{aligned} \tag{S20}$$

The total Berry connection now reads $\tilde{\boldsymbol{\mathcal{A}}}_\nu = \boldsymbol{\mathcal{A}}_\nu + \boldsymbol{\mathcal{A}}_\nu^{(1)}$. One direct consequence of the field induced Berry connection is the Berry curvature also acquires a field correction given by $\boldsymbol{\Omega}_\nu^{(1)} = \nabla_{\mathbf{k}}\times\boldsymbol{\mathcal{A}}_\nu^{(1)}$.

The second term of $\boldsymbol{\mathcal{A}}_\nu^{(1)}$ can be rewritten with components

$$\mathrm{Re}\sum_{\mu\neq\nu}\left[(\mathbf{B}\times\partial_{\mathbf{k}})_l\mathcal{A}^l_{\mu\nu}\boldsymbol{\mathcal{A}}_{\nu\mu}\right]_i=\mathrm{Re}\sum_{\mu\neq\nu}\epsilon_{jkl}B_j\partial_k\mathcal{A}^l_{\mu\nu}\mathcal{A}^i_{\nu\mu}=\epsilon_{jkl}\partial_k g_\nu^{li}B_j, \tag{S21}$$

where $g_\nu^{ij}=\mathrm{Re}\sum_{\mu\neq\nu}\mathcal{A}^i_{\nu\mu}\mathcal{A}^j_{\mu\nu}$ is the quantum metric. By substituting Eq. (S14), magnetic field induced Berry connection thus reads

$$\begin{aligned}\mathcal{A}_\nu^{(1),i}&=2\mathrm{Re}\sum_{\mu\neq\nu}\mathcal{A}^i_{\nu\mu}\mathcal{C}_{\mu\nu}-\frac{e}{2\hbar}\epsilon_{jkl}\partial_k g_\nu^{li}B_j\\&=-2\mathrm{Re}\sum_{\mu\neq\nu}\frac{\mathcal{A}^i_{\nu\mu}B_j m^j_{\mu\nu}}{\varepsilon_\nu-\varepsilon_\mu}-\frac{e}{2\hbar}\epsilon_{jkl}\partial_k g_\nu^{li}B_j\\&=-2\mathrm{Re}\sum_{\mu\neq\nu}\frac{\mathcal{A}^i_{\nu\mu}m^j_{\mu\nu}}{\varepsilon_\nu-\varepsilon_\mu}B_j-\frac{e}{2\hbar}\epsilon_{jkl}\partial_k g_\nu^{li}B_j.\end{aligned} \tag{S22}$$

By introducing a novel quantum geometric quantities, the magnetoelectric tensor $\mathbf{F}_\nu$, the field induced Berry connection $\boldsymbol{\mathcal{A}}_\nu^{(1)}$ can be reexpressed as

$$\mathcal{A}_\nu^{(1),i}=F_\nu^{ij}B_j. \tag{S23}$$

where $F_\nu^{ij}$ is given by

$$F_\nu^{ij}=-2\mathrm{Re}\sum_{\mu\neq\nu}\frac{\mathcal{A}^i_{\nu\mu}m^j_{\mu\nu}}{\varepsilon_\nu-\varepsilon_\mu}-\frac{e}{2\hbar}\epsilon_{jkl}\partial_k g_\nu^{li}. \tag{S24}$$

We also note that the term $\epsilon_{jkl}\partial_k g_\nu^{li}$ can be rewritten as

$$\epsilon_{jkl}\partial_k g_\nu^{li}=\frac{1}{2}\epsilon_{jkl}(\partial_k g_\nu^{li}-\partial_l g_\nu^{ki})=\frac{1}{2}\epsilon_{jkl}(\partial_i g_\nu^{kl}+\partial_k g_\nu^{li}-\partial_l g_\nu^{ki})=\epsilon_{jkl}\Gamma_\nu^{lki}, \tag{S25}$$

where we have used the identity $\epsilon_{jkl}\partial_i g_\nu^{kl}=0$. Here,

$$\Gamma_\nu^{lki}=\frac{1}{2}(\partial_i g_\nu^{kl}+\partial_k g_\nu^{li}-\partial_l g_\nu^{ki}) \tag{S26}$$

is referred to as the quantum Christoffel symbol. Now, $F_\nu^{ij}$ is written as

$$F_\nu^{ij}=-2\mathrm{Re}\sum_{\mu\neq\nu}\frac{\mathcal{A}^i_{\nu\mu}m^j_{\mu\nu}}{\varepsilon_\nu-\varepsilon_\mu}-\frac{e}{2\hbar}\epsilon_{jkl}\Gamma_\nu^{lki}. \tag{S27}$$

### B. Electric field induced correction of orbital magnetic moment

Since the term $e\mathbf{E}\cdot\boldsymbol{\mathcal{A}}_\nu^{(1)}=e\mathbf{E}\cdot\mathbf{F}_\nu\cdot\mathbf{B}$ represents an energy shift of the wave packet, it follows that $e\mathbf{E}\cdot\mathbf{F}_\nu$ correspond to the correction of orbital magnetic moment induced by the electric field. This interpretation provides the rationale for referring to $\mathbf{F}_\nu$ [Eq. (S27)] as the magnetoelectric tensor. Therefore, the total magnetic moment is given by

$$\tilde{\mathbf{m}}_\nu=\mathbf{m}_\nu+e\mathbf{E}\cdot\mathbf{F}_\nu. \tag{S28}$$

### C. Gauge invariant formalisms

We now convert quantum geometric quantities in previous section to the gauge invariant form. First, the quantum metric reads

$$\begin{aligned}g_\nu^{ij}&=\mathrm{Re}\sum_{\mu\neq\nu}\mathcal{A}^i_{\nu\mu}\mathcal{A}^j_{\mu\nu}\\&=\mathrm{Re}\sum_{\mu\neq\nu}\langle\nu|i\partial_i|\mu\rangle\langle\mu|i\partial_j|\nu\rangle\\&=\mathrm{Re}\sum_{\mu\neq\nu}\frac{\langle\nu|\partial_i\mathcal{H}|\mu\rangle\langle\mu|\partial_j\mathcal{H}|\nu\rangle}{(\varepsilon_\nu-\varepsilon_\mu)^2}.\end{aligned} \tag{S29}$$

Subsequently, the orbital magnetic moment vector reads

$$\mathbf{m}_\nu = \frac{e}{2\hbar}\mathrm{Im}\sum_{\mu\neq\nu}\boldsymbol{\mathcal{A}}_{\nu\mu}\times\boldsymbol{\mathcal{A}}_{\mu\nu}(\varepsilon_\mu-\varepsilon_\nu), \tag{S30}$$

which can be corresponded to an antisymmetric tensor

$$\begin{aligned} m_\nu^{ij} &= \epsilon_{ijk}m_\nu^k \\ &= \epsilon_{ijk}\epsilon_{klr}\frac{e}{2\hbar}\mathrm{Im}\sum_{\mu\neq\nu}\mathcal{A}^l_{\nu\mu}\mathcal{A}^r_{\mu\nu}(\varepsilon_\mu-\varepsilon_\nu) \\ &= \epsilon_{ijk}\epsilon_{klr}\frac{-e}{2\hbar}\mathrm{Im}\sum_{\mu\neq\nu}\langle\nu|\partial_i|\mu\rangle\langle\mu|\partial_j|\nu\rangle(\varepsilon_\mu-\varepsilon_\nu) \\ &= (\delta_{il}\delta_{jr}-\delta_{ir}\delta_{jl})\frac{-e}{2\hbar}\mathrm{Im}\sum_{\mu\neq\nu}\frac{\langle\nu|\partial_l\mathcal{H}|\mu\rangle\langle\mu|\partial_r\mathcal{H}|\nu\rangle}{\varepsilon_\nu-\varepsilon_\mu} \\ &= -\frac{e}{\hbar}\mathrm{Im}\sum_{\mu\neq\nu}\frac{\langle\nu|\partial_i\mathcal{H}|\mu\rangle\langle\mu|\partial_j\mathcal{H}|\nu\rangle}{\varepsilon_\nu-\varepsilon_\mu}. \end{aligned} \tag{S31}$$

We can collect these results as

$$\begin{cases} g_\nu^{ij} = \mathrm{Re}\sum_{\mu\neq\nu}\dfrac{\langle\nu|\partial_i\mathcal{H}|\mu\rangle\langle\mu|\partial_j\mathcal{H}|\nu\rangle}{(\varepsilon_\nu-\varepsilon_\mu)^2}, \\ m_\nu^{ij} = -\dfrac{e}{\hbar}\mathrm{Im}\sum_{\mu\neq\nu}\dfrac{\langle\nu|\partial_i\mathcal{H}|\mu\rangle\langle\mu|\partial_j\mathcal{H}|\nu\rangle}{\varepsilon_\nu-\varepsilon_\mu}. \end{cases} \tag{S32}$$

The orbital magnetic moment $m_\nu^{ij}$ is antisymmetric about indices $\{i,j\}$, while the quantum metric $g_\nu^{ij}$ is symmetric.

Additionally, for magnetoelectric tensor $\mathbf{F}_\nu$ [Eq. (S27)], we only focus on the inter-band orbital magnetic moment part because we have already obtained the gauge invariant form of quantum metric $\mathbf{g}_\nu$. The element of inter-band orbital magnetic moment reads [Eq. (S15)]

$$\begin{aligned} m^j_{\mu\nu} =& \frac{e}{2}\epsilon_{jkl}\sum_{\rho\neq\nu}(v^k_{\mu\rho}+v^k_\nu\delta_{\rho\mu})\mathcal{A}^l_{\rho\nu} \\ =& \frac{e}{2\hbar}\epsilon_{jkl}\left[\sum_{\rho\neq\nu}\langle\mu|\partial_k\mathcal{H}|\rho\rangle\langle\rho|i\partial_l|\nu\rangle+\langle\nu|\partial_k\mathcal{H}|\nu\rangle\langle\mu|i\partial_l|\nu\rangle\right] \\ =& \frac{ie}{2\hbar}\epsilon_{jkl}\left[\sum_{\rho\neq\nu}\frac{\langle\mu|\partial_k\mathcal{H}|\rho\rangle\langle\rho|\partial_l\mathcal{H}|\nu\rangle}{\varepsilon_\nu-\varepsilon_\rho}+\frac{\langle\nu|\partial_k\mathcal{H}|\nu\rangle\langle\mu|\partial_l\mathcal{H}|\nu\rangle}{\varepsilon_\nu-\varepsilon_\mu}\right]. \end{aligned} \tag{S33}$$

The magnetoelectric tensor is thus given by

$$\begin{aligned} F_\nu^{ij} &= -2\mathrm{Re}\sum_{\mu\neq\nu}\frac{\mathcal{A}^i_{\nu\mu}m^j_{\mu\nu}}{\varepsilon_\nu-\varepsilon_\mu}-\frac{e}{2\hbar}\epsilon_{jkl}\Gamma_\nu^{lki} \\ &= -2\mathrm{Re}\sum_{\mu\neq\nu}\frac{\langle\nu|i\partial_i|\mu\rangle m^j_{\mu\nu}}{\varepsilon_\nu-\varepsilon_\mu}-\frac{e}{2\hbar}\epsilon_{jkl}\Gamma_\nu^{lki} \\ &= -2\mathrm{Re}\sum_{\mu\neq\nu}\frac{-i\langle\nu|\partial_i\mathcal{H}|\mu\rangle m^j_{\mu\nu}}{(\varepsilon_\nu-\varepsilon_\mu)^2}-\frac{e}{2\hbar}\epsilon_{jkl}\Gamma_\nu^{lki} \\ &= -2\mathrm{Im}\sum_{\mu\neq\nu}\frac{\langle\nu|\partial_i\mathcal{H}|\mu\rangle m^j_{\mu\nu}}{(\varepsilon_\nu-\varepsilon_\mu)^2}-\frac{e}{2\hbar}\epsilon_{jkl}\Gamma_\nu^{lki}. \end{aligned} \tag{S34}$$

## SII. CALCULATION OF DISTRIBUTION FUNCTION

For the electron evolution in the phase-space, it is desirable to introduce the non-equilibrium distribution function $f(\mathbf{r}, \mathbf{k}, t)$, which satisfies [8]

$$\frac{\partial f}{\partial t} + \dot{\mathbf{r}} \cdot \nabla f + \dot{\mathbf{k}} \cdot \frac{\partial f}{\partial \mathbf{k}} = \mathcal{I}\{f\}. \tag{S35}$$

where $\mathcal{I}\{f\}$ is the deviation of distribution function due to collisions. At the steady state, $\partial_t f = 0$. For a uniform perturbation, we drop the spatial gradient term. Now, the distribution function $f$ satisfies

$$\dot{\mathbf{k}} \cdot \frac{\partial f}{\partial \mathbf{k}} = \mathcal{I}\{f\}. \tag{S36}$$

It is the celebrated Boltzmann equation. The left side is called drift term, while the right side is collision term. It is usually assumed that the non-equilibrium distribution deviates less from the equilibrium distribution. We shall assume a simple relaxation time approximation

$$\mathcal{I}\{f\} \simeq -\frac{f - f_0}{\tau}, \tag{S37}$$

where $f_0$ is the Fermi-Dirac distribution function, and $\tau$ is the relaxation time.

Now, under the electric field, i.e., $\dot{\mathbf{k}} = -e\mathbf{E}/\hbar$, the Boltzmann equation becomes

$$\begin{aligned} &\frac{-e}{\hbar}\mathbf{E} \cdot \partial_{\mathbf{k}} f = -\frac{f - f_0}{\tau}, \\ \Rightarrow \quad &\left(1 - \frac{\tau e}{\hbar}\mathbf{E} \cdot \partial_{\mathbf{k}}\right) f = f_0, \\ \Rightarrow \quad &(1 - \mathcal{Q}) f = f_0, \end{aligned} \tag{S38}$$

where the operator $\mathcal{Q}$ is defined as $\mathcal{Q} \equiv (\tau e/\hbar)\mathbf{E} \cdot \partial_{\mathbf{k}}$. Accordingly, we can obtain the solution as

$$f = \frac{1}{1 - \mathcal{Q}} f_0 = \sum_{a=0}^{\infty} \mathcal{Q}^a f_0. \tag{S39}$$

The zeroth-order term is just $f_0$, the first-order and second-order terms are evidently

$$\begin{cases} f_1 = \dfrac{\tau e}{\hbar}\mathbf{E} \cdot \partial_{\mathbf{k}} f_0, \\ f_2 = \left(\dfrac{\tau e}{\hbar}\mathbf{E} \cdot \partial_{\mathbf{k}}\right)^2 f_0, \end{cases} \tag{S40}$$

while the $a$-th order term is given by

$$f_a = \mathcal{Q}^a f_0 = \left(\frac{\tau e}{\hbar}\mathbf{E} \cdot \partial_{\mathbf{k}}\right)^a f_0. \tag{S41}$$

Explicitly, by using the non-equilibrium distribution function, we have the response of a measurable quantity $\mathcal{S}$ as

$$\mathcal{R} = \frac{1}{\mathcal{V}} \sum_{\nu, \mathbf{k}} \langle \mathcal{S} \rangle f = \int [d\mathbf{k}] \langle \mathcal{S} \rangle f, \tag{S42}$$

where $\mathcal{R}$ represents response, and $[d\mathbf{k}]$ represents $\sum_\nu d^d\mathbf{k}/(2\pi)^d$ with dimension $d$ and band index $\nu$.

## SIII. CALCULATION OF NONLINEAR MAGNETIZATION COEFFICIENT

According to definition, the orbital magnetization is given by

$$\mathbf{M} = \int [d\mathbf{k}] \tilde{\mathbf{m}}_\nu f. \tag{S43}$$

The total orbital magnetic moment $\tilde{\mathbf{m}}_\nu$ has two origins, the first is the intrinsic orbital magnetic moment of the Bloch state, and the second is the anomalous correction linear in the electric field

$$\tilde{\mathbf{m}}_\nu = \mathbf{m}_\nu + \mathbf{m}_\nu^{(1)} = \mathbf{m}_\nu + e\mathbf{F}_\nu \cdot \mathbf{E}. \tag{S44}$$

Here, $\mathbf{m}_\nu$ is the intra-band orbital magnetic moment given by

$$m_\nu^i = -\epsilon_{ijk}\frac{e}{\hbar}\mathrm{Im}\sum_{\mu\neq\nu}\frac{\langle\nu|\partial_j\mathcal{H}|\mu\rangle\langle\mu|\partial_k\mathcal{H}|\nu\rangle}{\varepsilon_\nu-\varepsilon_\mu} \tag{S45}$$

with full anti-symmetric tensor $\epsilon_{ijk}$, which is time-reversal odd, i.e., $\mathcal{T}^\dagger m_\nu^i(\mathbf{k})\mathcal{T} = -m_\nu^i(-\mathbf{k})$. The quantity $\mathbf{F}_\nu$ is the magnetoelectric tensor given by Eq. (S34) [for convenience, to allow contraction between the column index of $\mathbf{F}_\nu$ and the electric field, $\mathbf{F}_\nu$ used here is actually the transpose of that in Eq. (S34)]

$$F_\nu^{ij} = -2\mathrm{Im}\sum_{\mu\neq\nu}\frac{m_{\nu\mu}^i\langle\mu|\partial_j\mathcal{H}|\nu\rangle}{(\varepsilon_\nu-\varepsilon_\mu)^2} - \frac{e}{2\hbar}\epsilon_{ikl}\Gamma_\nu^{lkj}, \tag{S46}$$

which is time-reversal odd, i.e., $\mathcal{T}^\dagger F_\nu^{ij}(\mathbf{k})\mathcal{T} = -F_\nu^{ij}(-\mathbf{k})$, where $\mathbf{m}_{\mu\nu}$ is the inter-band element of the orbital magnetic moment [Eq. (S33)]

$$m_{\mu\nu}^i = \frac{ie}{2\hbar}\epsilon_{ijk}\left[\sum_{\rho\neq\nu}\frac{\langle\mu|\partial_j\mathcal{H}|\rho\rangle\langle\rho|\partial_k\mathcal{H}|\nu\rangle}{\varepsilon_\nu-\varepsilon_\rho} + \frac{\langle\nu|\partial_j\mathcal{H}|\nu\rangle\langle\mu|\partial_k\mathcal{H}|\nu\rangle}{\varepsilon_\nu-\varepsilon_\mu}\right], \tag{S47}$$

and $g_\nu^{ij}$ is the quantum metric tensor given by Eq. (S29)

$$g_\nu^{ij} = \mathrm{Re}\sum_{\mu\neq\nu}\frac{\langle\nu|\partial_i\mathcal{H}|\mu\rangle\langle\mu|\partial_j\mathcal{H}|\nu\rangle}{(\varepsilon_\nu-\varepsilon_\mu)^2}, \tag{S48}$$

which is time-reversal even, i.e., $\mathcal{T}^\dagger g_\nu^{ij}(\mathbf{k})\mathcal{T} = g_\nu^{ij}(-\mathbf{k})$.

Up to the second order of electric field, the distribution function is expanded as Eq. (S40),

$$f = f_0 + \frac{\tau e}{\hbar}\mathbf{E}\cdot\partial_\mathbf{k} f_0 + \left(\frac{\tau e}{\hbar}\mathbf{E}\cdot\partial_\mathbf{k}\right)^2 f_0. \tag{S49}$$

Considering the correction of energy [2, 4, 5], the Fermi distribution function $f_0$ is now a function of electric field $\mathbf{E}$. To obtain the nonlinear response, we expand $f_0$ as a series

$$f_0(\varepsilon_\nu + \frac{e^2}{2}\mathbf{E}\cdot\boldsymbol{\mathcal{G}}_\nu\cdot\mathbf{E}) \simeq f_0(\varepsilon_\nu) + \frac{e^2}{2}\mathbf{E}\cdot\boldsymbol{\mathcal{G}}_\nu\cdot\mathbf{E}f_0', \tag{S50}$$

where $\boldsymbol{\mathcal{G}}_\nu$ is the the band-normalized quantum metric given by

$$\mathcal{G}_\nu^{ij} = 2\mathrm{Re}\sum_{\mu\neq\nu}\frac{\langle\nu|\partial_i\mathcal{H}|\mu\rangle\langle\mu|\partial_j\mathcal{H}|\nu\rangle}{(\varepsilon_\nu-\varepsilon_\mu)^3}, \tag{S51}$$

which is a time-reversal even tensor, i.e., $\mathcal{T}^\dagger\mathcal{G}_\nu^{ij}(\mathbf{k})\mathcal{T} = \mathcal{G}_\nu^{ij}(-\mathbf{k})$.

By substituting the expression of $f$ [Eq. (S82)] into Eq. (S43) and retaining terms up to the square of the electric field, we can obtain that

$$\begin{aligned} M_i &= \int[d\mathbf{k}]\tilde{m}_\nu^i f \\ &= \int[d\mathbf{k}](m_\nu^i + eF_\nu^{ij}E_j)\Big[f_0 + \frac{e^2}{2}\mathcal{G}_\nu^{jk}E_jE_kf_0' + \frac{\tau e}{\hbar}E_j\partial_j f_0 + \Big(\frac{\tau^2e^2}{\hbar^2}E_jE_k\partial_j\partial_k\Big)f_0\Big] \\ &= \int[d\mathbf{k}]\Big[m_\nu^i\big(f_0 + \frac{e^2}{2}\mathcal{G}_\nu^{jk}f_0'E_jE_k + \frac{\tau e}{\hbar}\partial_j f_0E_j + \frac{\tau^2e^2}{\hbar^2}\partial_j\partial_k f_0E_jE_k\big) + eF_\nu^{ij}f_0E_j + eF_\nu^{ij}\frac{\tau e}{\hbar}\partial_k f_0E_jE_k\Big]. \end{aligned} \tag{S52}$$

According to the order of electric field $\mathbf{E}$, the orbital magnetization $\mathbf{M}$ can be divided into three contributions, the first is the orbital magnetization of ground state

$$M_i^{(0)} = \int[d\mathbf{k}]m_\nu^i f_0, \tag{S53}$$

which vanishes with time-reversal symmetry. The second contribution is linear to the electric field $\mathbf{E}$, which reads

$$\begin{aligned} M_i^{(1)} &= \int [d\mathbf{k}] \Big( m_\nu^i \frac{\tau e}{\hbar} \partial_j f_0 + e F_\nu^{ij} f_0 \Big) E_j \\ &= \int [d\mathbf{k}] \big( m_\nu^i \tau e v_\nu^j f_0' + e F_\nu^{ij} f_0 \big) E_j, \end{aligned} \tag{S54}$$

where $\mathbf{v}_\nu = \partial_{\mathbf{k}} \varepsilon_\nu / \hbar$, and only the first term retains with time-reversal symmetry. The third contribution is a nonlinear response which is in second order of electric field, given by

$$\begin{aligned} M_i^{(2)} &= \int [d\mathbf{k}] \Big[ m_\nu^i \Big( \frac{e^2}{2} \mathcal{G}_\nu^{jk} f_0' + \frac{\tau^2 e^2}{\hbar^2} \partial_j \partial_k f_0 \Big) + e F_\nu^{ij} \frac{\tau e}{\hbar} \partial_k f_0 \Big] E_j E_k \\ &= \int [d\mathbf{k}] \Big[ m_\nu^i \Big( \frac{e^2}{2} \mathcal{G}_\nu^{jk} f_0' + \frac{\tau^2 e^2}{\hbar} \partial_j v_\nu^k f_0' \Big) + \tau e^2 F_\nu^{ij} v_\nu^k f_0' \Big] E_j E_k, \end{aligned} \tag{S55}$$

where, under time-reversal symmetry, only the last term remains.

In summary, for the system with time-reversal symmetry, i.e., non-magnetic system, the linear and nonlinear orbital magnetization coefficients are given by

$$\begin{cases} \alpha_{ij} = \tau e \displaystyle\int [d\mathbf{k}] m_\nu^i v_\nu^j f_0', \\ \alpha_{ijk} = \tau e^2 \displaystyle\int [d\mathbf{k}] F_\nu^{ij} v_\nu^k f_0'. \end{cases} \tag{S56}$$

## SIV. PARTICLE-HOLE SYMMETRY AND SOLO OF QUANTUM CHRISTOFFEL SYMBOL

### A. Two-band system

For a two-band system, the Hamiltonian can be written as $\mathcal{H} = d_0 + \mathbf{d} \cdot \boldsymbol{\sigma}$, where $\sigma_i$'s are the Pauli matrices. The eigenenergies are given by $\varepsilon_\pm = d_0 \pm d$, with $d = \sqrt{d_x^2 + d_y^2 + d_z^2}$. The corresponding eigenstates are denoted by $|\pm\rangle$. We first calculate the quantity

$$\langle + | \partial_i \mathcal{H} | - \rangle \langle - | \partial_j \mathcal{H} | + \rangle. \tag{S57}$$

One notes that the quantum geometry quantities do not depend on the trivial term $d_0$. This is because the trivial term is an overall $\mathbf{k}$-dependent energy shift for both bands, and according to Eq. (S32), they are not affected by such overall shift (except for the magnetoelectric tensor $\mathbf{F}_\nu$). Therefore, the kinetic velocity operator can be simply written as

$$\partial_i \mathcal{H} = \partial_i d_l \sigma_l, \tag{S58}$$

corresponding matrix element is given by

$$\langle + | \partial_i \mathcal{H} | - \rangle = \partial_i d_l \langle + | \sigma_l | - \rangle. \tag{S59}$$

We thus have

$$\langle + | \partial_i \mathcal{H} | - \rangle \langle - | \partial_j \mathcal{H} | + \rangle = (\partial_i d_l)(\partial_j d_r) \langle + | \sigma_l | - \rangle \langle - | \sigma_r | + \rangle. \tag{S60}$$

Additionally, by using the complete condition, an identity can be proved as

$$\begin{aligned} \langle + | \sigma_l | - \rangle \langle - | \sigma_r | + \rangle &= \big[ \langle + | \sigma_l | - \rangle \langle - | \sigma_r | + \rangle + \langle + | \sigma_l | + \rangle \langle + | \sigma_r | + \rangle \big] - \langle + | \sigma_l | + \rangle \langle + | \sigma_r | + \rangle \\ &= \langle + | \sigma_l \big[ | - \rangle \langle - | + | + \rangle \langle + | \big] \sigma_r | + \rangle - \frac{d_l d_r}{d^2} \\ &= \langle + | \sigma_l \sigma_r | + \rangle - \frac{d_l d_r}{d^2} \\ &= \langle + | (i \epsilon_{lrs} \sigma_s + \delta_{lr}) | + \rangle - \frac{d_l d_r}{d^2} \\ &= \delta_{lr} - \frac{d_l d_r}{d^2} + i \epsilon_{lrs} \frac{d_s}{d}, \end{aligned} \tag{S61}$$

where we have used an identity for the product of two Pauli matrices

$$\sigma_l \sigma_r = i\epsilon_{lrs}\sigma_s + \delta_{lr}, \tag{S62}$$

and the relation

$$\langle \pm|\sigma_l|\pm\rangle = \pm\frac{d_l}{d}. \tag{S63}$$

Similarly, for the valence band, we have

$$\langle -|\sigma_l|+\rangle\langle +|\sigma_r|-\rangle = \delta_{lr} - \frac{d_l d_r}{d^2} - i\epsilon_{lrs}\frac{d_s}{d}. \tag{S64}$$

For the quantum metric we only need the real part of Eq. (S61)

$$\mathrm{Re}\langle +|\sigma_l|-\rangle\langle -|\sigma_r|+\rangle = \delta_{lr} - \frac{d_l d_r}{d^2}. \tag{S65}$$

Thus, the quantum metric for the upper band is given by

$$\begin{aligned} g_+^{ij} &= \frac{\mathrm{Re}\langle +|\partial_i \mathcal{H}|-\rangle\langle -|\partial_j \mathcal{H}|+\rangle}{(\varepsilon_+ - \varepsilon_-)^2} \\ &= (\partial_i d_l)(\partial_j d_r)\Big(\delta_{lr} - \frac{d_l d_r}{d^2}\Big)\frac{1}{4d^2} \\ &= \frac{1}{4d^2}\Big[\partial_i \mathbf{d}\cdot\partial_j \mathbf{d} - \frac{1}{d^2}(\partial_i \mathbf{d}\cdot\mathbf{d})(\partial_j \mathbf{d}\cdot\mathbf{d})\Big], \end{aligned} \tag{S66}$$

and for the lower band $g_-^{ij} = g_+^{ij}$. For the orbital magnetic moment, we only need the imaginary part of Eq. (S61)

$$\mathrm{Im}\langle +|\sigma_l|-\rangle\langle -|\sigma_r|+\rangle = \epsilon_{lrs}\frac{d_s}{d}. \tag{S67}$$

Then, the orbital magnetic moment for upper band reads

$$\begin{aligned} m_+^{ij} &= -\frac{e}{\hbar}\frac{\mathrm{Im}\langle +|\partial_i \mathcal{H}|-\rangle\langle -|\partial_j \mathcal{H}|+\rangle}{\varepsilon_+ - \varepsilon_-} \\ &= -\frac{e}{\hbar}\frac{1}{2d}(\partial_i d_l)(\partial_j d_r)\epsilon_{ijk}\frac{d_k}{d} \\ &= -\frac{e}{\hbar}\frac{(\partial_i \mathbf{d}\times\partial_j \mathbf{d})\cdot\mathbf{d}}{2d^2}, \end{aligned} \tag{S68}$$

while for the lower band $m_-^{ij} = m_+^{ij}$. Assembling these results, we have

$$\begin{cases} g_\pm^{ij} = \dfrac{1}{4d^2}\Big[\partial_i \mathbf{d}\cdot\partial_j \mathbf{d} - \dfrac{1}{d^2}(\partial_i \mathbf{d}\cdot\mathbf{d})(\partial_j \mathbf{d}\cdot\mathbf{d})\Big], \\ m_\pm^{ij} = -\dfrac{e}{\hbar}\dfrac{(\partial_i \mathbf{d}\times\partial_j \mathbf{d})\cdot\mathbf{d}}{2d^2}. \end{cases} \tag{S69}$$

They are consistent with Ref. [3].

Similarly, from Eq. (S27), the magnetoelectric tensor reads

$$\begin{aligned} F_+^{ij} &= -\frac{e}{\hbar}\epsilon_{jkl}\mathrm{Re}\Big[\frac{\langle +|\partial_i \mathcal{H}|-\rangle\langle -|\partial_k \mathcal{H}|-\rangle\langle -|\partial_l \mathcal{H}|+\rangle}{(\varepsilon_+ - \varepsilon_-)^3} + \frac{\langle +|\partial_i \mathcal{H}|-\rangle\langle +|\partial_k \mathcal{H}|+\rangle\langle -|\partial_l \mathcal{H}|+\rangle}{(\varepsilon_+ - \varepsilon_-)^3}\Big] - \frac{e}{2\hbar}\epsilon_{jkl}\partial_k g_+^{li} \\ &= -\frac{e}{\hbar}\epsilon_{jkl}\Big[\partial_k d_0 - \frac{(\partial_k d_r)d_r}{d} + \partial_k d_0 + \frac{(\partial_k d_r)d_r}{d}\Big]\frac{1}{2d}\frac{\mathrm{Re}\langle +|\partial_i \mathcal{H}|-\rangle\langle -|\partial_l \mathcal{H}|+\rangle}{(\varepsilon_+ - \varepsilon_-)^2} - \frac{e}{2\hbar}\epsilon_{jkl}\partial_k g_+^{li} \\ &= -\frac{e}{\hbar}\epsilon_{jkl}\frac{\partial_k d_0}{d}g_+^{li} - \frac{e}{2\hbar}\epsilon_{jkl}\partial_k g_+^{li}, \end{aligned} \tag{S70}$$

where the two-band expression of quantum metric [Eq. (S66)] has been used, while for the lower band

$$F_-^{ij} = \frac{e}{\hbar}\epsilon_{jkl}\frac{\partial_k d_0}{d}g_+^{li} - \frac{e}{2\hbar}\epsilon_{jkl}\partial_k g_+^{li}. \tag{S71}$$

Here, we have restored the trivial term $d_0$ of Hamiltonian, which is effective only for diagonal elements of kinetic operator, i.e.,

$$\begin{cases} \langle\pm|\partial_i\mathcal{H}|\pm\rangle = \partial_i d_0 + \partial_i d_l\langle\pm|\sigma_l|\pm\rangle = \partial_i d_0 \pm \dfrac{(\partial_i d_l)d_l}{d}, \\ \langle+|\partial_i\mathcal{H}|-\rangle = \partial_i d_0\langle+|-\rangle + \partial_i d_l\langle+|\sigma_l|-\rangle = \partial_i d_l\langle+|\sigma_l|-\rangle. \end{cases} \tag{S72}$$

Thus, the final result reads

$$F_\pm^{ij} = \mp\frac{e}{\hbar}\epsilon_{jkl}\frac{\partial_k d_0}{d}g_+^{li} - \frac{e}{2\hbar}\epsilon_{jkl}\partial_k g_+^{li}. \tag{S73}$$

### B. 2D massive Dirac model

The four-band Hamiltonian of 2D massive Dirac model is

$$\begin{aligned}\mathcal{H} &= v(k_x\tau_x\sigma_x + k_y\tau_x\sigma_y) + m\tau_z \\ &= \begin{bmatrix} m & 0 & 0 & v(k_x - ik_y) \\ 0 & m & v(k_x+ik_y) & 0 \\ 0 & v(k_x-ik_y) & -m & 0 \\ v(k_x+ik_y) & 0 & 0 & -m \end{bmatrix},\end{aligned} \tag{S74}$$

where $v, m$ are model parameters, and $\tau$ and $\sigma$ denote two independent sets of Pauli matrices. This model preserves time-reversal symmetry, $\mathcal{T} = \sigma_y K$, and can be block-diagonalized into two decoupled sectors via a unitary transformation

$$\begin{aligned}\mathcal{H} &\to \begin{bmatrix} m & v(k_x-ik_y) & 0 & 0 \\ v(k_x+ik_y) & -m & 0 & 0 \\ 0 & 0 & m & v(k_x+ik_y) \\ 0 & 0 & v(k_x-ik_y) & -m \end{bmatrix} \\ &= \begin{bmatrix} h_+ & 0 \\ 0 & h_- \end{bmatrix}.\end{aligned} \tag{S75}$$

For time-reversal even mechanisms [Eq. (S56)], it is sufficient to consider only one of the branches of Hamiltonian related by time-reversal symmetry, which reads

$$h_+ = v(k_x\sigma_x + k_y\sigma_y) + m\sigma_z. \tag{S76}$$

This implies that the quantum geometric quantities for the model in Eq. (S74) can be evaluated using the results derived from the two-band case [Eq. (S73)].

## SV. SYMMETRY ANALYSIS AND 2D MATERIAL CANDIDATES

The electric-field-induced magnetization is characterized by the magnetization coefficient $\boldsymbol{\alpha}$ as

$$M_i = \alpha_{ij}E_j + \alpha_{ijk}E_jE_k, \tag{S77}$$

where $(i, j, k)$ represent Cartesian coordinates and the Einstein's summation convention is implied. The coefficient $\alpha_{ij}$ characterizes linear response, and $\alpha_{ijk}$ characterizes nonlinear response.

For systems with inversion symmetry $\mathcal{P}$, the linear response is strictly forbidden because the moment vector is an axial vector, which remains invariant under inversion. For the time-reversal symmetry $\mathcal{T}$, the restriction to the response coefficients depends on the parity of the powers of the relaxation time $\tau$. The detailed forms of $\boldsymbol{\alpha}$ constrained by symmetries $\mathcal{P}$ and $\mathcal{T}$ are presented in Table S1.

For system with time-reversal symmetry, i.e., non-magnetic system, all intrinsic contributions $\propto \tau^0$ vanishes identically. This is the case that we shall discuss in this work. Additionally, this $\mathcal{T}$-even nonlinear magnetization generation coefficient $\alpha_{ijk}$ must preserves the point group symmetry

$$\alpha_{i'j'k'} = \det(\mathcal{O})\mathcal{O}_{i'i}\mathcal{O}_{j'j}\mathcal{O}_{k'k}\alpha_{ijk}, \tag{S78}$$

where $\mathcal{O}$ is representation matrix for the point group operation in Cartesian coordinate. Assuming the polar configuration, i.e., the electric field applying along the $\hat{x}$ or $\hat{y}$ direction, the point group symmetry constraints are listed in Table S2.

2D material candidates that satisfy the symmetry conditions for a non-vanishing $\alpha_{zxx}$ are listed in Table S3.

TABLE S1. Constraints on magnetization coefficient from $\mathcal{P}$, $\mathcal{T}$ and $\mathcal{PT}$ symmetries. ✓(✗) means that the symmetry operation is allowed (forbidden), and $n = 0, 1, 2, \cdots$.

| | $\mathcal{P}$ | $\mathcal{T}$ | $\mathcal{PT}$ |
|---|---|---|---|
| $\alpha_{ij} \propto \tau^{2n}$ | ✗ | ✗ | ✓ |
| $\alpha_{ij} \propto \tau^{2n+1}$ | ✗ | ✓ | ✗ |
| $\alpha_{ijk} \propto \tau^{2n}$ | ✓ | ✗ | ✗ |
| $\alpha_{ijk} \propto \tau^{2n+1}$ | ✓ | ✓ | ✓ |

TABLE S2. Constraints on nonlinear magnetization coefficient from point group symmetries. ✓(✗) means that the symmetry operation is allowed (forbidden). The improper rotation $\mathcal{S}_i^n$ can be readily obtained by $\mathcal{S}_i^n = \mathcal{C}_i^n \mathcal{M}_i$, where $n = 3, 4, 6$ and $i$ represents the Cartesian coordinate.

| | $\mathcal{C}_z^2$ | $\mathcal{C}_z^3$ | $\mathcal{C}_z^{4,6}$ | $\mathcal{C}_x^{2,4,6}$ | $\mathcal{C}_y^{2,4,6}$ | $\mathcal{C}_x^3$ | $\mathcal{C}_y^3$ | $\mathcal{M}_z$ | $\mathcal{M}_x$ | $\mathcal{M}_y$ |
|---|---|---|---|---|---|---|---|---|---|---|
| $\alpha_{xxx}$ | ✗ | ✓ | ✗ | ✓ | ✗ | ✓ | ✓ | ✗ | ✓ | ✗ |
| $\alpha_{zzz}$ | ✓ | ✓ | ✓ | ✗ | ✗ | ✓ | ✓ | ✓ | ✗ | ✗ |
| $\alpha_{xyy}$ | ✗ | ✓ | ✗ | ✓ | ✗ | ✓ | ✗ | ✗ | ✓ | ✗ |
| $\alpha_{zxx}$ | ✓ | ✓ | ✓ | ✗ | ✗ | ✗ | ✓ | ✓ | ✗ | ✗ |

## SVI. COMPARISON WITH SPIN CONTRIBUTION

### A. Nonlinear spin magnetization

Similar to the orbital contribution, the spin magnetization is given by the integral of the spin moment $\tilde{\mathbf{m}}_\nu$ carried by the Bloch states weighted by the distribution function $f$, which is written as

$$\mathbf{M} = \int [d\mathbf{k}] \tilde{\mathbf{m}}_\nu f. \tag{S79}$$

The total spin moment $\tilde{\mathbf{m}}_\nu$ has two origins, the first is the expectation value of the spin operator for the Bloch state, and the second is the electric-field correction

$$\tilde{\mathbf{m}}_\nu = \mathbf{m}_\nu + \mathbf{m}_\nu^{(1)} = -g\mu_B \langle \nu | \mathbf{s} | \nu \rangle + e\mathbf{F}_\nu \cdot \mathbf{E}, \tag{S80}$$

where $g$ is the Landé g factor for spin, $\mu_B = e\hbar/(2m)$ is the Bohr magneton, $\mathbf{s} = \boldsymbol{\sigma}/2$ is the dimensionless spin operator, $-e$ is the electron charge, $m$ is the electron mass, and $\mathbf{F}_\nu$ is the spin magnetoelectric tensor given by [6]

$$F_\nu^{ij} = 2g\mu_B \mathrm{Im} \sum_{m \neq n} \frac{\langle \nu | s_i | \mu \rangle \langle \mu | \partial_j \mathcal{H} | \nu \rangle}{(\varepsilon_\nu - \varepsilon_\mu)^2}, \tag{S81}$$

which is a time-reversal odd tensor, i.e., $\mathcal{T}^\dagger F_\nu^{\mathrm{S},ij}(\mathbf{k}) \mathcal{T} = -F_\nu^{\mathrm{S},ij}(-\mathbf{k})$.

Up to the second order of electric field, the distribution function is given by [Eq. (S40)]

$$f = f_0 + \frac{\tau e}{\hbar} \mathbf{E} \cdot \partial_{\mathbf{k}} f_0 + \left( \frac{\tau e}{\hbar} \mathbf{E} \cdot \partial_{\mathbf{k}} \right)^2 f_0. \tag{S82}$$

Considering the correction of energy [2, 4, 5], the Fermi distribution function $f_0$ is now a function of electric field $\mathbf{E}$. To obtain the nonlinear response, we expand $f_0$ as a series

$$f_0(\varepsilon_\nu + \frac{e^2}{2} \mathbf{E} \cdot \boldsymbol{\mathcal{G}}_\nu \cdot \mathbf{E}) \simeq f_0(\varepsilon_\nu) + \frac{e^2}{2} \mathbf{E} \cdot \boldsymbol{\mathcal{G}}_\nu \cdot \mathbf{E} f_0', \tag{S83}$$

where $\boldsymbol{\mathcal{G}}_\nu$ is the the band-normalized quantum metric given by Eq. (S51).

TABLE S3. 2D material candidates that could host $\alpha_{zxx}$, the second-order nonlinear magnetization polarized along the $z$ direction induced by an $x$-direction $ac$ electric field, based on a search in the open computational database 2DMatPedia [9] of 2D materials. The point groups 1 and $\bar{1}$ are discarded.

| Point group | Candidates |
|---|---|
| 4 | $TiPb_9O_{11}$ |
| $\bar{4}$ | $Sn_3(HO_2)_2$, $AgBrO_4$, $NaI_3O_8$ |
| $4/m$ | $Ru_4Se_5$, $Te_5Ru_4$, $Os_4Se_5$, $Ru_4S_5$, $Ta_4O_9$, $Nb_4O_9$, $Zr(IO_3)_4$, $AgXeF_9$, $CaTi_4O_9$, $AgPb_4ClO_4$, $NbVO_5$, $VPO_5$, $MgTi_4O_9$ |
| 3 | $B_2Te$, $In_2Se$, $Al_2Se$, $In_2Te$, $Ga_2Te$, $In_2Se$, $In_2Te$, $Ga_2Te$, $B_2Se$, $Al_2Se$, $B_2Se$, $Tl_2Te$, $Tl_2Se$, $Al_2S$, $Ga_2S$, $Ga_2S$, $Tl_2Se$, $In_2S$, $B_2S$, $In_2S$, $Tl_2S$, $CuBi(PSe_3)_2$, $TlV_3(SeO_6)_2$, $KV_3(SeO_6)_2$, $LiSnCl_3$, $AgBi(PSe_3)_2$, $RbV_3(SeO_6)_2$, $Tl_2S$ |
| $\bar{3}$ | $BiF_3$, $Al_2Te$, $S_4O_9$, $Al_2Te$, $ZnI_2$, $P_2Pd$, $NiAs_2$, $Se_4O_9$, $HgCl_2$, $HgI_2$, $HgF_2$, $Zn(ReO_4)_2$,$Pt(NO_3)_2$, $SnPS_3$, $Zr_3SO_9$, $Te_4O_9$, $FeSn_2(CN)_6$, $Tl_2Sn(AsS_3)_2$, $Rb_2Sn(H_2N)_6$, $Na_2H_6PtO_6$, $Li_3SbS_3$, $Tl(IO_3)_3$, $LuBiO_3$, $TiSnO_3$, $BiSbO_3$, $Sc(IO_3)_3$, $Mg(ReO_4)_2$, $Bi_{14}Te_{13}S_8$, $SbN_9$, $Re_3(TeBr)_7$, $TmBiO_3$, $YBiO_3$, $TiGeO_3$, $AsI_3$, $FePb_2(CN)_6$, $CdPSe_3$, $ErBiO_3$, $HgBr_2$, $Li_3BiS_3$, $Li_3Sb_2(PO_4)_3$, $In(IO_3)_3$, $HoBiO_3$ |
| 6 | – |
| $\bar{6}$ | $Ge_3Sb_2O_9$, $Si_3Bi_2O_9$, $AgNO_3$, $Si_3Sb_2O_9$, $Ge_3Bi_2O_9$ |
| $6/m$ | – |

By substituting the expression of $f$ [Eq. (S82)] into Eq. (S79), and retaining terms up to the square of the electric field, we can obtain that

$$\begin{aligned} M_i &= \int [d\mathbf{k}] \tilde{m}_\nu^{\mathrm{S},i} f \\ &= \int [d\mathbf{k}] (-g\mu_B s_\nu^i + eF_\nu^{ij} E_j) \Big[ f_0 + \frac{e^2}{2} \mathcal{G}_\nu^{jk} E_j E_k f_0' + \frac{\tau e}{\hbar} E_j \partial_j f_0 + \Big( \frac{\tau^2 e^2}{\hbar^2} E_j E_k \partial_j \partial_k \Big) f_0 \Big] \\ &= \int [d\mathbf{k}] \Big[ - g\mu_B s_\nu^i \big( f_0 + \frac{e^2}{2} \mathcal{G}_\nu^{jk} f_0' E_j E_k + \frac{\tau e}{\hbar} \partial_j f_0 E_j + \frac{\tau^2 e^2}{\hbar^2} \partial_j \partial_k f_0 E_j E_k \big) + eF_\nu^{ij} f_0 E_j + eF_\nu^{ij} \frac{\tau e}{\hbar} \partial_k f_0 E_j E_k \Big], \end{aligned} \tag{S84}$$

where we have denoted $s_\nu^i = \langle \nu | s_i | \nu \rangle$. According to the order of electric field $\mathbf{E}$, the spin moment density $\mathbf{M}$ can be divided into three contributions, the first is the spin magnetization of ground state

$$M_i^{\mathrm{S},(0)} = -g\mu_B \int [d\mathbf{k}] s_\nu^i f_0, \tag{S85}$$

which vanishes with time-reversal symmetry. The second contribution is linear to the electric field, given by

$$\begin{aligned} M_i^{(1)} &= \int [d\mathbf{k}] \Big[ (-g\mu_B s_\nu^i) \frac{\tau e}{\hbar} \partial_j f_0 + e F_\nu^{ij} f_0 \Big] E_j \\ &= \int [d\mathbf{k}] \big[ (-g\mu_B s_\nu^i) \tau e v_\nu^j f_0' + e F_\nu^{ij} f_0 \big] E_j, \end{aligned} \tag{S86}$$

where $\mathbf{v}_\nu = \partial_\mathbf{k} \varepsilon_\nu / \hbar$, and only the first term retains with time-reversal symmetry. The third contribution is a nonlinear response which is in second order of electric field, given by

$$\begin{aligned} M_i^{(2)} &= \int [d\mathbf{k}] \Big[ (-g\mu_B s_\nu^i) \Big( \frac{e^2}{2} \mathcal{G}_\nu^{jk} f_0' + \frac{\tau^2 e^2}{\hbar^2} \partial_j \partial_k f_0 \Big) + e F_\nu^{ij} \frac{\tau e}{\hbar} \partial_k f_0 \Big] E_j E_k \\ &= \int [d\mathbf{k}] \Big[ (-g\mu_B s_\nu^i) \Big( \frac{e^2}{2} \mathcal{G}_\nu^{jk} f_0' + \frac{\tau^2 e^2}{\hbar} \partial_j v_\nu^k f_0' \Big) + \tau e^2 F_\nu^{ij} v_\nu^k f_0' \Big] E_j E_k, \end{aligned} \tag{S87}$$

where, under time-reversal symmetry, only the last term remains.

In summary, for the system with time-reversal symmetry, i.e., non-magnetic system, the linear and nonlinear spin magnetization coefficients are given by

$$\begin{cases} \alpha_{ij} = -g\mu_B \tau e \int [d\mathbf{k}] s_\nu^i v_\nu^j f_0', \\ \alpha_{ijk} = \tau e^2 \int [d\mathbf{k}] F_\nu^{ij} v_\nu^k f_0'. \end{cases} \tag{S88}$$

### B. First principle calculations for $BiF_3$

Using the same first-principles calculation method as in the main text, we have evaluated the spin contribution [Eq. (S88)] to the nonlinear magnetization. As shown in Fig. S1, the spin contribution is negligibly small over two orders of magnitude weaker than the orbital contribution.

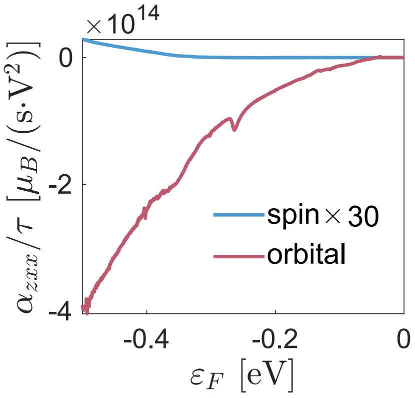


FIG. S1. Calculated $\alpha_{zxx}$ for $BiF_3$ as a function of the Fermi energy $\varepsilon_F$. The blue and red curves represent spin (×30 for visibility) and orbital contributions, respectively.


[1] D. Xiao, M.-C. Chang, and Q. Niu, Berry phase effects on electronic properties, Rev. Mod. Phys. **82**, 1959 (2010).

[2] Y. Gao, S. A. Yang, and Q. Niu, Field Induced Positional Shift of Bloch Electrons and Its Dynamical Implications, Phys. Rev. Lett. **112**, 166601 (2014).

[3] A. Graf and F. Piéchon, Berry curvature and quantum metric in $N$-band systems: An eigenprojector approach, Phys. Rev. B **104**, 085114 (2021).

[4] C. Wang, Y. Gao, and D. Xiao, Intrinsic Nonlinear Hall Effect in Antiferromagnetic Tetragonal CuMnAs, Phys. Rev. Lett. **127**, 277201 (2021).

[5] H. Liu, J. Zhao, Y.-X. Huang, W. Wu, X.-L. Sheng, C. Xiao, and S. A. Yang, Intrinsic Second-Order Anomalous Hall Effect and Its Application in Compensated Antiferromagnets, Phys. Rev. Lett. **127**, 277202 (2021).

[6] C. Xiao, W. Wu, H. Wang, Y.-X. Huang, X. Feng, H. Liu, G.-Y. Guo, Q. Niu, and S. A. Yang, Time-Reversal-Even Nonlinear Current Induced Spin Polarization, Phys. Rev. Lett. **130**, 166302 (2023).

[7] H. Wang, Y.-X. Huang, H. Liu, X. Feng, J. Zhu, W. Wu, C. Xiao, and S. A. Yang, Orbital Origin of the Intrinsic Planar Hall Effect, Phys. Rev. Lett. **132**, 056301 (2024).

[8] H. Haug and A.-P. Jauho, *Quantum kinetics in transport and optics of semiconductors*, Vol. 2 (Springer, 2008).

[9] J. Zhou, L. Shen, M. D. Costa, K. A. Persson, S. P. Ong, P. Huck, Y. Lu, X. Ma, Y. Chen, H. Tang, *et al.*, 2DMatPedia, an open computational database of two-dimensional materials from top-down and bottom-up approaches, Sci. Data **6**, 86 (2019).
